# Supplementary material for: Generating Robust Counterfactual Witnesses for Graph Neural Networks
Source: arXiv:2404.19519 source file (2024-04-30)
Supplement: Supplementary file 1 [file cr-appendix.tex]

\section{Proofs and Algorithms}
\label{sec-appendix}

%\subsection{Proofs for Verification Problems}

\eat{
We start by proving Lemma~\ref{lm-verifyw} 
and Lemma~\ref{lm-verifycw} as two tractable cases 
for the verification problem of 
explanations. Before this, 
We first show the following claim. 

\vspace{.5ex}
\noindent
\textbf{Claim}: \textit{For a deterministic, fixed \gnn model $\M$ and a graph $G$ with test node set 
$V_T$, the inference cost, \ie the 
time cost of inference process $M(V_T, G)$ is in \PTIME. }

We exploit the time cost analysis of 
the inference process of representative 
classes of \gnns~\cite{chen2020scalable,zhou2021accelerating}.  
It has been shown in formal analysis that 
the time cost of the 
inference function $M$, 
which performs a fixed point, 
terminating message-passing process, is determined by 
$L$, $|V|$, $|E|$, $d$, and $F$, 
where $L$ is the number of layers of the \gnn
$\M$, $d$ = $\frac{|E|}{|V|}$ is the average degree of $G$, and $F$ is the number of features per node. 
For example, the inference cost 
of representative message-passing based \gnns (\eg \gcns, \gats, \gsage), or PageRank based \ppnps are in
$O(L|E|F+L|V|F^2)$~\cite{chen2020scalable,zhou2021accelerating}. Given that 
$\M$ is fixed, the inference process 
does not change. 
Given that $\M$ is deterministic, 
it ensures that the time cost 
of $M(V_T, G)$ for a given 
set of $V_T$ over $G$ is 
in \PTIME.

\stitle{Proof of Lemma~\ref{lm-verifyw}}.
 The witness verification is in \PTIME.

\begin{proof}
We provide a \PTIME algorithm, 
denoted as \verifyw, for 
the witness verification problem. 
By definition, it suffices to verify, for 
each node $v\in V_T$ with $M(v, G)$ = $l$, 
if $M(v, G_s)$ = $l$. To this end, 
\verifyw simply performs the inference process of \gnn $M$ over $G_s$, which takes as input the node features $X$, 
%\textcolor{red}{[AK: $X$ in bold, to be consistent with notations in ''Graph Neural Networks (GNNs)'' paragraph, Section II?] - now seems we are not using bold for X 
%consistently} 
but a revised adjacency matrix %$A_s$ 
with entries ``flipped'' to $0$ 
if the corresponding edges are not in $G_s$. 
As $M$ is a fixed deterministic 
model, the inference cost is in \PTIME. 
As $M$ is a fixed deterministic 
model, given the 
aforementioned \textbf{Claim}, the inference cost is in \PTIME. 
\end{proof}

\stitle{Proof of Lemma~\ref{lm-verifycw}}. 
\textit{The verification for \cw is in \PTIME.} 

\begin{proof}
We provide a second procedure, 
denoted as \verifycw, as a constructive 
proof. By definition, it performs the 
following. (1) It constructs 
a graph $G'$ = $G\setminus G_s$.  
%by disturbing all the edges 
%of $G_s$ (while keeping all the nodes). 
(2) For each node 
$v\in V_T$ with assigned label $l$, 
(a) it first invokes \verifyw to 
verify if $G_s$ is a factual witness of $M(v,G)$, 
in \PTIME; 
and (b) If so, it invokes \verifyw to check if $M(v, G')\neq l$. 
If $G_s$ fails the test at any 
node $v\in V_T$, it returns no. 
Otherwise, $G_s$ is a \cw for 
$V_T$. As \verifyw is in \PTIME (Lemma~\ref{lm-verifyw}), 
\verifycw remains to be in \PTIME. 
\end{proof}
}

\eat{
We first prove that 
for any node $v\in V_T$, 
a $k$-\rcw $G_w$ for $M(v,G)$ 
remains to be a $k'$-\rcw 
for $M(v,G)$, for any $k'\in[0,k]$. 
%\textcolor{red}{[AK: $M(v,G)$ not defined in the statement of Lemma 1].}
One can verify the above result by contradiction. 
Assume that there is a $k'\in [0,k]$, such that 
a $k$-\rcw $G_s$ is not a $k'$-\rcw, then 
(a) $G_w$ is not a factual witness, or 
it is not counterfactual, both contradict 
to that $G_w$ is an \rcw; 
or (b) $G_w$ is a \cw but is not robust. Then there exists a $k'$-disturbance with $k'$ edges $E_k'$ in 
$G\setminus G_w$, which 
``disproves'' that $G_w$ is a $k$-\rcw. As $k'\leq k$, 
the same $k'$-disturbance prevents $G_w$ to be a $k$-\rcw by definition. 
This contradicts to that $G_w$ is a $k$-\rcw. 
Hence, $G_w$ remains to be a 
$k'$-\rcw for $M(v,G)$. 
As the test node $v$ ranges over 
$V_T$, the above analysis holds 
to verify that $G_w$ remains to be a 
$k'$-\rcw for any subset 
$V_T'\subseteq V_T$. 
Lemma~\ref{lm-k} thus follows. 
}

\eat{
\stitle{Proof of Theorem~\ref{lm-rwverify}}. 
\textit{The $k$-\rcw verification is \NP-hard.} 

\begin{proof} 
We show the above result by proving that 
when $M$ is any fixed model from \ppnps, 
and when $V_T$ contains only a single test node $v$,  
the $k$-\rcw verification is already \NP-hard. 
Before we present the formal proof, 
we first review several 
notations we shall use. 

\eetitle{Notations}. 
(1) \ppnps~\cite{gasteiger2018predict} are a class of 
Personalized PageRank based 
\gnns $\M$. The Personalized PageRank matrix is defined as: $\Pi = (1-\alpha)(I-\alpha\Hat{D}^{-1} \Hat{A})^{-1}$~\cite{bojchevski2019certifiable}. Here  $D$ is the diagonal matrix of node out-degrees with ${D}_{i i}=\sum_{j} {A}_{i j}$, and $\alpha$ is teleport probability. 
% \warn{give the 
% update function as the personalized pagerank}. 
(2) Given a fixed \ppnps $M$, 
 % over a set of links $L$. 
a node $v\in V_T$ is 
{\em certifiably robust}~\cite{bojchevski2019certifiable}, % \wrt configuration $C$, 
if its ``worst-case margin'' 
$m_{l, *}^{*}(v)$ = $\min_{c \neq l}$ $m_{l, c}^{*}(v)>0$,
where $M(v, G)$ = $l$ is the true label of $v$, 
and $c$ is any other label $(c\neq l)$. Here 
$m_{l, c}^{*}(v)$ is defined as: 
\begin{equation}
\label{eq-margin-1}
\begin{split}
\vspace{-2.5ex}
m_{l, c}^{*}(v) &=\min _{E_k \subseteq G\setminus G_s} m_{l, c}(v)\\
& =\min_{E_k \subseteq G\setminus G_s} \pi_{E_k}\left(v\right)^{T}\left(Z_{\{:, l\}}-Z_{\{:, c\}}\right)
\vspace{-1ex}
\end{split}
\end{equation}

where $E_k$ ranges over all the possible 
$k$-disturbances that can be applied to $G'$ = 
$G\setminus G_s$, and ${\pi_{E_k}\left(v\right) =\boldsymbol{\Pi}_{v,:}}$ is the PageRank vector of node $v$ in the PageRank matrix $\boldsymbol{\Pi}=(1-\alpha)({I}_{N}-\alpha {D}^{-1} {A'})^{-1}$, 
with $A'$ obtained by 
disturbing the adjacency matrix of $G$ 
 with $E_k$, \eg $A'[i,j]$ = $0$ (resp. $1$) if 
$(v_i, v_j)\in E_k$ (resp. $(v_i, v_j)\not\in E_k$)\footnote{
We  
do not explicitly change $G$ 
or $G'$, but represent the tentative disturbing 
by ``fliping'' the entries of $A$ to obtain 
a ``disburbed'' counterpart $A'$.}. 
By verifying $m_{l, *}^{*}(v) > 0$, \ie $m_{l, c}^{*}(v) > 0$ for any $c\in \text{\L}$ $(c\neq l)$, it indicates that under any $k$-disturbance in $G\setminus G_s$, $M$ always  
infers a correct   
label $l$ to $v$ given its output $Z$. 

\vspace{.5ex}
We now prove that for a given subgraph 
$G_s$ of $G$ with $V_T$ contains a single node $v$, 
and a fixed \gnn $M$ that is a \ppnps, 
the verification is already \NP-hard. To see this, 
an algorithm may first invoke \verifyw and \verifycw to determine if $G_s$ is a \cw. If $G_s$ is neither a factual witness nor a \cw, one can safely conclude that $G_s$ is not a $k$-\rcw. 
This process remains to be in \PTIME (Lemma~\ref{lm-verifyw} 
and Lemma~\ref{lm-verifycw}). 

It next suffices to verify 
that testing a \cw $G_s$ is a $k$-\rcw 
for $v$ is \NP-hard. 
We prove this by first showing that it is {\em a 
general case} of the decision version of the $k$-edge PageRank maximization (\kmp). \kmp is to find 
at most $k$ node pairs $E_{k}$ from a graph %$G\setminus G_s$, 
s.t. the PageRank scores of a %set of nodes 
%$V_T$ 
 a targeted node $v$ 
is maximized if $k$ links are inserted. 
For this, 
we refer the readers to 
the detailed proof of Lemma~\ref{lm-condition-iff}. 

We next show that 
\kmp is \NP-hard. We consider the decision version of \kmp:

\begin{small}
\begin{mdframed}
\textbf{Given}: A graph $G_=(V, E)$, 
%a subgraph $G_s$, 
a node $v \in V$, a budget number $k$, and a target PageRank score $\theta$.

\sstab
\textbf{Problem}: Is there a set of $k$ edges $E_k$ in %$G\setminus G_s$ 
$G$, 
s.t. PageRank score of $v$ after inserting $E_k$ is at least $\theta$?
\end{mdframed}
\end{small}

We then show the hardness of \kmp by constructing a \PTIME reduction from link building problem (\lbp), a known \NP-hard problem~\cite{olsen2014approximability}. 
The decision problem of \lbp is: % of the following form:

\begin{small}
\begin{mdframed}
\textbf{Given}: A graph $G=(V, E)$, a node $v_x \in V$, a budget number $k \geq 1$, and a target PageRank score $\theta$.

\sstab
\textbf{Problem}: Is there a set $S \subseteq V \backslash\{v_x\}$ with $|S|=k$ s.t. PageRank score of $x$ is at least $\theta$ in $G'(V, E \cup(S \times\{v_x\}))$?
\end{mdframed}
\end{small}

Utilizing the graph $G(V, E)$ from \lbp, 
the target node $v_x$ corresponds to the subset $V_T=\{v_x\}$ in the simplest case of \kmp, 
directly translating the single-node optimization to a set-based context. 
Each edge in $S \times \{v_x\}$ is considered an insertion edge in $E_k$. 
The objective in both problems aligns, aiming for a PageRank score of at least $\theta$ with $k$ edge insertions. In our setting, $G_s$ is initialized and expanded from $V_T$, so $V_T \subseteq G_s$.

If there's a solution to the \lbp, we can identify a set $S \subseteq V \backslash\{v_x\}$ with $|S|=k$ s.t. adding edges from every node in $S$ to the node $v_x$ results in an increment in $v_x$'s PageRank Score to at least $\theta$. 
This outcome directly contributes to forming a set $E_k = S \times \{v_x\}$ for \kmp. 
Given that $V_T = \{v_x\}$, the insertion of edges in $E_k$ into the graph ensures that the PageRank scores for $V_T$ also achieve or exceed the threshold $\theta$.

Conversely, if there is a solution exists for \kmp, where the addition of $k$ edges in $E_k$ into $G\setminus G_s$ increases in PageRank scores for $V_T$ to at least $\theta$, given $V_T = \{v_x\}$, it indicates that the specific arrangement of insertion edges $E_k$ effectively maximizes $v_x$'s PageRank score. This maximization is in a manner akin to the solution set $S$ in \lbp. This implies the solution to the \lbp is affirmative.

Therefore, this reduction shows that solving \kmp encapsulates the complexity of solving \lbp, since \lbp is \NP-hard~\cite{olsen2014approximability}, the $k$-\rcw verification problem is also \NP-hard.
\end{proof}
}
%By definition, a \cw $G_s$ is a $k$-\rcw of $M(v, G)=l$ if and only if for {\em any} graph $\hat{G}$ of $G$ obtained by a {\em $k$-disturbance} on $G\setminus G_s$, $G_s$ remains to be a \cw for $M(v,\hat{G})$=$l$. 
%Observe that the latter is exactly characterized as 
%``node certifiable robustness'' in~\cite{bojchevski2019certifiable}. 
%That is, the $k$-\rcw verification problem is {\em equivalent} to the problem of deciding whether a test node $v$ is certifiably robust. 

\eat{
\begin{proof}
We make a case for \ppnps.  
To determine if a given graph $G_s$ is a $k$-\rcw, we first invoke \verifyw and \verifycw to determine if $G_s$ is a \cw. If $G_s$ is neither a factual witness nor a \cw, we can safely conclude that $G_s$ is not a $k$-\rcw. 
Otherwise, the problem equals to verify if a \cw $G_s$ is a $k$-\rcw. 
By definition, a subgraph $G_s$ is a $k$-\rcw of $M(v, G)=l$ if for {\em any} graph $\widetilde{G}$ of $G$ obtained by a {\em $k$-disturbance} on $G\setminus G_s$, $G_s$ remains to be a \cw for $M(v,\widetilde{G})$=$l$. 
The disturbance here includes both insertion and removal.
To ensure the robustness of $G_s$, it should remain to be a \cw when subjected to $k$ most hostile edge. 
Based on this intuition, as derived by~\cite{bojchevski2019certifiable}, the $k$-\rcw verification problem is equivalent to a $k$-edge Maximum PageRank Optimization Problem (\kmp), which means that we are aiming to find $k$ disturbance edges $E_{k}$ from $G\setminus G_s$, s.t. PageRank scores of $V_T$ are maximized. We will prove this in Lemma~\ref{lm-condition-iff}.

We start with a special case focusing on edge insertion. Given a graph $G$, whether inserting $k$ edges s.t. PageRank scores of $V_T$ can be maximized. We show its decision version:

\begin{small}
\begin{mdframed}
\textbf{Given}: A graph $G=(V, E)$, a subgraph $G_s$, a set of nodes $V_T \subseteq V$, a budget number $k$, and a target PageRank score $\theta$.

\sstab
\textbf{Question}: Is there a set of $k$ edges $E_k$ from $G\setminus G_s$ s.t. PageRank scores of $V_T$ after inserting $E_k$ are at least $\theta$?
\end{mdframed}
\end{small}

We then show the hardness of \kmp by performing a \PTIME reduction from the link Building Problem(\lbp), a known \NP-hard problem~\cite{olsen2014approximability}, which is defined in its decision version as:

\begin{small}
\begin{mdframed}
\textbf{Given}: A graph $G=(V, E)$, a node $x \in V$, a budget number $k \geq 1$, and a target PageRank score $\theta$.

\sstab
\textbf{Question}: Is there a set $S \subseteq V \backslash\{x\}$ with $|S|=k$ s.t. PageRank score of $x$ is at least $\theta$ in $G'(V, E \cup(S \times\{x\}))$?
\end{mdframed}
\end{small}

Utilizing the graph $G(V, E)$ from \lbp, 
the target node $x$ corresponds to the subset $V_T=\{x\}$ in the simplest case of \kmp, 
directly translating the single-node optimization to a set-based context. 
Each edge in $S \times \{x\}$ is considered an insertion edge in $E_k$. 
The objective in both problems aligns, aiming for a PageRank score of at least $\theta$ with $k$ edge insertions. In our setting, $G_s$ is initialized and expanded from $V_T$, so $V_T \subseteq G_s$.

If there's a solution to the \lbp, we can identify a set $S \subseteq V \backslash\{x\}$ with $|S|=k$ s.t. adding edges from every node in $S$ to the node $x$ results in an increase in $x$'s PageRank Score to at least $\theta$. 
This outcome directly contributes to forming a set $E_k = S \times \{x\}$ for \kmp. 
Given that $V_T = \{x\}$, the insertion of edges in $E_k$ into the graph ensures that the PageRank scores for $V_T$ also achieve or exceed the threshold $\theta$.

Conversely, if there is a solution exists for \kmp, where the addition of $k$ edges in $E_k$ into $G\setminus G_s$ increases in PageRank scores for $V_T$ to at least $\theta$, given $V_T = \{x\}$, it indicates that the specific arrangement of insertion edges $E_k$ effectively maximizes $x$'s PageRank score. This maximization is in a manner akin to the solution set $S$ in \lbp. This implies the solution to the \lbp is affirmative.

Therefore, this reduction shows that solving \kmp encapsulates the complexity of solving \lbp, since \lbp is \NP-Hard~\cite{olsen2014approximability}, the $k$-\rcw verification problem is also \NP-Hard.
\end{proof}
}

\begin{algorithm}[tb!]

    \caption{Algorithm \verifyrcw (single node)} %Extendable
%    \scriptsize
    \begin{algorithmic}[1]
        \REQUIRE A configuration $C$ = $\{G, G_s, v, \M, k\}$; \\
        \ENSURE  \kw{true} if $G_s$ is a 
        $k$-\rcw; \kw{false} otherwise. \\
         \IF{$\verifyw(C)$ = \kw{false}} 
        \STATE \textbf{return} \kw{false}; 
        \ENDIF
        \STATE construct graph $G'$ := $G\setminus G_s$; 
        \IF{$\verifycw(G',C)$ = \kw{false}}
        \STATE \textbf{return} \kw{false}; \ENDIF
        \STATE $\hat{A}^\prime$ := $A^\prime + I$, where $A^\prime$ is adjacency matrix of $G'$;
        \FOR{$j = 1$ to $k$}
            \STATE 
            construct all distinct $j$-disturbances $E_j$; 
            \FOR{each $E_j$}
            \STATE
            flip $\hat{A}^\prime$ and update $G'$ (implicitly); 
            \IF{$\verifycw(G',C)$ = \kw{false}} 
            \STATE \textbf{return} \kw{false}; 
            \ENDIF
            \STATE restore $\hat{A}^\prime$ and $G'$; 
            \ENDFOR
            \ENDFOR
            \eat{
            \IF{$\verifyrcw(C, G_I, j)$ = \kw{true}}
                 \IF{j=$k$} 
                    \STATE \textbf{return} $G_I$; 
                 \ELSE  \STATE \textbf{continue}; 
                \ENDIF
            \ELSE \STATE $G_I$:=$G_s$; \textbf{break}; 
           % \textbf{continue};  
            \ENDIF
            \ENDFOR
       \STATE \textbf{return} $G_s$; 
       }
      \STATE \textbf{return} \kw{true};  
    \end{algorithmic}
    \label{procedure:verifyrcw}
   % \vspace{-1ex}
\end{algorithm}

\eat{
\stitle{Verification of $k$-\rcw}.  
We introduce a general verification 
algorithm, denoted as \verifyrcw (illustrated 
in Algorithm~\ref{procedure:verifyrcw}). 

Given a configuration $C$, 
the algorithm first invokes \verifyw and \verifycw to 
check if $G_s$ is a factual witness and a \cw, 
both in \PTIME (Lemma~\ref{lm-verifyw} and Lemma~\ref{lm-verifycw}). 
If $G_s$ remains to be a \cw, 
it next performs a 
$k$-round of verification, 
to verify if $G_s$ is an 
$j$-\rcw in the $j$-th round. 
%\warn{explain ``bitmap''}. 
The disturbed adjacancy matrix $\hat{A}$ is encoded and maintained as a bitmap for memory-efficiency. 
It {\em early terminates} whenever 
a $j$-th disturbance is 
identified, which already disproves that 
$G_s$ is a $k$-\rcw (Lemma~\ref{lm-k}). }

\stitle{Analysis of Algorithm \ref{procedure:verifyrcw} %$k$-\rcw
}. 
The algorithm~\verifyrcw always terminates: it performs at most 
$k$ rounds of permutation 
and verification processes; in each round, 
all $j$-disturbances ($j\in[0,k]$) are 
investigated and verified 
to check if $G_s$ remains to be a \cw. The 
algorithm correctly 
returns ``true'' or 
``false'' ensured by 
the \verifycw, which is 
in \PTIME. 
The overall time cost is thus in hence in 
$O(|G\setminus G_s|^k)$ time. 
\eat{
\warn{add 
(1) correctness analysis: 
1. show it eventually terminates; and 2. 
that it correctly output ``true'' or 
``false''. 
(2) Give time cost analysis. 
This verification is a simple 
enumeration and verify process, 
which explores all possible 
$k$-disturbances, hence in 
$O(|G\setminus G_s|^k)$ time}.  
}

%\verifyrcw

\eat{
\stitle{Proof of Theorem~\ref{lm-rwverify-tractable}}.  
\textit{Given the configuration $C$ that specifies 
\ppnp $\M$, and when only $(k,b)$-disturbances are allowed, the verification problem for $k$-\rcw is in \PTIME.  }

As a constructive proof,  
we present the detailed 
correctness and the time cost analysis 
for the algorithm \verifyrcwp.  
Below we first present a detailed proof 
for Lemma~\ref{lm-condition-iff} as 
a building block in our analysis.

%\vspace{-1ex}
\eetitle{Proof of Lemma~\ref{lm-condition-iff}}. 
%\warn{continue here}. 
Given the configuration $C$ %= $(G,G_s, V_T, \M, k)$ 
that specifies 
\ppnp $\M$, and when only $(k,b)$-disturbance is 
allowed, let $G_s$ be a verified \cw of $M(v,G)$ = $l$ 
for a node $v\in V_T$, then 
$G_s$ is a $k$-\rcw of $M(v,G)$=$l$,  
if and only if $M(v, G\setminus E^*_k)$ = $l$, 
where $E^*_k$ = $\argmax_{E_k\subseteq G\setminus G_s, c\neq l}, (\textbf{Z}_{\{:,c\}}-\textbf{Z}_{\{:,l\}})^T\pi_{E_k}\left(v\right)$.

\begin{proof}
Let $\widetilde{G}$ be the graph 
obtained by disturbing $E^*_k$ in 
$G\setminus G_s$. 

\stitle{(If)}: We show the 
following If statement: 
Given $C$, \ppnp $\M$, under $(k,b)$-disturbances, let $G_s$ a \cw of $M(v,G)$ = $l$ for a node $v\in V_T$, 
if $M(v, G\setminus E^*_k)$ = $l$, 
where $E^*_k$ = $\argmax_{E_k\subseteq G\setminus G_s, c\neq l}, (\textbf{Z}_{\{:,c\}}-\textbf{Z}_{\{:,l\}})^T\pi_{E_k}\left(v\right)$, then 
$G_s$ is a $k$-\rcw of $M(v,G)$=$l$. 
To see this, 
%let $E^*_k$ be the node pairs to be disturbed in the corresponding 
%$(k,b)$-disturbance in $G\setminus G_s$. 
observe that $E^*_k$ maximizes 
$(Z_{\{:,c\}}-Z_{\{:,l\}})^T\pi_{E_k}\left(v\right)$, 
which indicates that it minimizes the gap between 
the likelihoods that {\em some} label $c\neq l$ being assigned to 
$v$, quantified by the worst-case margin 
$m^*_{l,c}$, for {\em every} label $c$ that 
is not $l$. That is, disturbing $E^*_k$ is
``most likely'' to change the 
current result $M(v,G)$=$l$, 
\ie $M(v,\widetilde{G})$=$c\neq l$, 
for any label $c\in L$. 
Then, if $m^*_{l,c}>0$ for every $c\neq l$ under 
disturbance $E^*_k$, $M(v, \widetilde{G})$ 
will remain to be $l$. 
This means that no $(k,b)$-disturbance in $G\setminus G_s$ will change $v$'s label. 
Meanwhile, since disturbing $E_k^*$ alone is not crucial enough to affect the outcome of $M$ on $v$, and as $G_s$ is a verified \cw for $M(v, G) = l$, so $M(v, G\setminus G_s) = c' \neq l$, $c'\in L$, then $M(v, \widetilde{G}\setminus G_s)\neq l$ holds for any $(k,b)$-disturbance.
Hence, $G_s$ is a $k$-\rcw of $M(v,G)$=$l$ by 
definition under 
$(k,b)$-disturbances. 

\stitle{(Only If)}. The \textbf{Only If} 
condition states the following:  
given $C$ and \ppnp $M$, and let 
$G_s$ be a $k$-\rcw of $M(v,G)$=$l$, 
then $M(v, G\setminus E^*_k)$ = $l$. 
Here $E^*_k$ = $\argmax_{E_k\subseteq G\setminus G_s, c\neq l}, (\textbf{Z}_{\{:,c\}}-\textbf{Z}_{\{:,l\}})^T\pi_{E_k}\left(v\right)$, \ie 
the optimal $(k,b)$-disturbance that is 
applied ``outside'' of $G_s$ in 
$G$ that can maximize the term 
$\argmax_{E_k\subseteq G\setminus G_s, c\neq l}, (\textbf{Z}_{\{:,c\}}-\textbf{Z}_{\{:,l\}})^T\pi_{E_k}\left(v\right)$. 
Observe that maximizing 
the term is equivalent to 
minimize the ``worst-case margin'' 
$m^*_{l,*}(v)$, which 
intuitively indicates that 
the $(k,b)$-disturbance 
$E^*_k$ is most likely to 
``flip'' the current 
(correct) label $l$ to 
a label $c$, 
with $c$ ranges over 
all the labels that are 
different from $l$. 
If $m^*_{l,*}(v)>0$, 
$E^*_k$ leads to 
a change of label at $v$ 
that is predicted by 
$M$.  

The \textbf{Only If} condition can be shown by 
contradiction. Assuming (1) there exists a 
$(k,b)$-disturbance  
$E^*_k$ that can maximize 
$\argmax_{E_k\subseteq G\setminus G_s, c\neq l}, (\textbf{Z}_{\{:,c\}}-\textbf{Z}_{\{:,l\}})^T\pi_{E_k}\left(v\right)$, 
such that 
$M(v, \widetilde{G})\neq l$, 
and (2) $G_s$ is still a $k$-\rcw 
of $M(v, G)$ = $l$. Since 
$\M$ is fixed and deterministic, 
$M(v, G_s)$ = $l$ is not 
affected by disturbing $E_k$ 
``outside'' of $G_s$. 
On the other hand, $M(v, \widetilde{G})\neq l$, 
hence $G_s$ is not a factual witness 
for $M(v, \widetilde{G})$ = $l$, 
and hence not a \cw for $M(v, \widetilde{G})$ = $l$. 
This violates the third condition 
in the definition of $k$-\rcw 
for $G$. Hence $G_s$ is not a $k$-\rcw 
of $M(v,G)$ = $l$. 
This contradicts to the assumption 
that $G_s$ is a $k$-\rcw of $M(v,G)$=$l$. 
Hence the \textbf{Only If} 
condition holds. 

Putting these together, Lemma~\ref{lm-condition-iff} 
follows. The above analysis also verifies that 
testing \rcw for a single node $v$ is 
equivalent to solving the decision 
problem of \kmp. 
\end{proof}

\stitle{Correctness of \verifyrcwp}. 
%\warn{1. show it always terminates; and 2. 
%show when it terminate, it correctly 
%verifies the if and only if 
%condition of Lemma~\ref{lm-condition-iff}}.
We show the correctness of~\verifyrcwp. 
(1) The algorithm \verifyrcwp terminates. 
To see this, observe that 
the process in lines 1-5 can be executed in 
\PTIME (Lemma~\ref{lm-verifyw} and Lemma~\ref{lm-verifycw}). 
The process at line~6 iterates at most $L$-1 rounds 
to verify if there exists a $(k,b)$-disturbance 
that may disapprove $G_s$ as a robust $\rcw$ 
by changing the result of $M$ 
from $l$ to $c\in L$. To this end, 
it invokes procedure~\pri that 
simulates a greedy-based policy iteration 
process, which correctly solves 
a special case of an instance of 
LBP under local budget $b$, when 
$M$ is specified as an \ppnp. 
(2) The algorithm \verifyrcwp can correctly verify if and only if condition in Lemma~\ref{lm-condition-iff}. 
Procedure \pri greedily improvements the node pairs set $E_k^*$ by activating or deactivating edges that increase the PageRank score, which is similar to selecting actions in Stochastic Shortest Path (SSP) problem that lead to the lowest cost or highest reward~\cite{hollanders2011policy}. It utilizes a policy iteration approach that converges to the optimal solution by iteratively making locally optimal decisions that lead to global optimization (line 5-7 in \pri), and return $E_k^*$ with maximal PageRank score when no improvements can be made~\cite{bojchevski2019certifiable}. 
More clearly, in our scenario, it returns the node pairs set that is most likely to hurt $G_s$ as a \cw for $M(v, G)=l$. By utilizing its ``greedy'' nature, it can be early terminated when the current $E_k^*$ is already disapproved $G_s$ as a $k$-\rcw (line 8 in \pri), which is verified by checking if $M(v, G\setminus E_k^*) = l$ holds under this $E_k^*$.
Given proved Lemma~\ref{lm-condition-iff}, it is sufficient to show that \verifyrcwp can correctly verify if $G_s$ is a $k$-\rcw.
 
 % \warn{Mengying: check if this 
 % makes sense or revise}. 
%the time cost analysis below}. 
 
% \warn{Mengying: update the 
% detailed analysis of the 
% time cost below}. 

For time cost, we define $G' = G\setminus G_s$ and $d_m$ as the maximum degree for nodes in $G'$. 
In Procedure \pri, we introduce a local budget $b$ for each node in $G'$, this reduces the number of possible evaluated node pairs set from $\frac{2^{|G'|}}{|G'|}$ (as proved by ~\cite{mansour2013complexity}) to $\prod_{v \in V}{|G'_v| \choose b}$, which already ensures Procedure \pri is in \PTIME. 
Moreover, since Procedure \pri requires at least one final decision regarding the activation or deactivation of an edge in $G'$ in each iteration, and this decision will not be reversed in later iterations, it guarantee that the greedy process in Procedure \pri converges to the optimal $E_k^*$ in at most $|G'|$ iterations~\cite{hollanders2011policy}. 
During each iteration, the algorithm incurs a ranking cost of $O(d_m\log d_m)$ to select top-$b$ edges for each node (line 5 in \pri), and a verification cost by inferring a specific \gnn $M$ (line 8 in \pri).
\verifyrcwp invokes Procedure \pri for each $c \in L\setminus \{l\}$. Hence, the total cost is $O(L|G'|\cdot(d_m\log d_m+ LF(|E|+|V|F)))$ for a \ppnps $\M$.

\eat{
\stitle{Time cost of \verifyrcwp}. 
For the time cost, 
we observe the following. 
(1) \verifyrcw verifies at most 
$k\times b$ disturbances by exploring 
at  most $k$ rounds of 
top $b$ edge selection process; and 
(2) both \verifyw and \verifycw 
remains to be in \PTIME under 
$(k,b)$-disturbance, 
following Lemma~\ref{lm-verifyw} and Lemma~\ref{lm-verifycw}. 
Thus the total cost is in 
$O(kbL^2F(|E|+|V|F))$ for representative 
\gnns (\gcns, \gats, \gsage, \ppnps), 
where $b$ (bounded by node degree) 
and $L$ (layers of \gnns) are typically small. 
}

Putting these together, algorithm~\verifyrcwp 
correctly verifies $k$-\rcw in 
\PTIME. 
Theorem~\ref{lm-rwverify-tractable} 
thus follows. 
}

\subsection{Proofs for Generation Problems}

\stitle{Proof of Theorem~\ref{thm-rcw-gen}}. 
\textit{Given a configuration $C$ = $(G, V_T, M, k)$, 
$k$-\rcw generation problem is co-\NP-hard.}

\begin{proof}
%It suffices to consider a ``single node''. 
A problem is co-\NP-hard if 
its complementary problem is 
\NP-complete. The decision problem of 
$k$-\rcw generation for  
a configuration $C$  = $(C, v, M, k)$ 
is to decide if there exists a subgraph 
$G_s$ such that for any $k$-disturbance, 
$G_s$ remains to be a \cw 
for $M(v, \widetilde{G})$=$l$, 
where $\widetilde{G}$ is obtained by 
disturbing $G$ with a $k$-disturbance 
(see Section~\ref{sec:pre}). 
The complementary problem 
of $k$-\rcw generation 
is to decide whether there exists  
no subgraph $G_s$ in $G$ that 
can be a $k$-\rcw for $v$ with a true label 
$l$. That is, it is to decide 
for any subgraph $G_s$, 
there exists 
some $k$-disturbance that 
``disapproves'' $G_s$ to be 
a $k$-\rcw. If so, 
the answer is ``true'' 
(hence the answer for 
$k$-\rcw is ``false'' as 
no $k$-\rcw exists); otherwise, 
its answer is ``false'' 
(hence the answer for 
$k$-\rcw is ``true'', \ie 
there exists at least one 
$k$-\rcw for $v$). 

We make a case for \ppnps, 
and show that the complementary problem 
of generating $k$-\rcw for 
a single test node $v$ is  
\NP-complete. 
(1) There is an \kw{NP} algorithm 
that non-deterministically guesses 
a subgraph $G_s$ and a $k$-disturbance, 
and invokes an inference process of 
$M$ over the disturbed graph, 
given $G$, $G_s$ and $k$-disturbance, 
in \PTIME.  
(2) The \NP-hardness follows from Theorem~\ref{lm-rwverify}, 
which shows that the verification problem of 
$k$-\rcw for \ppnps is already 
\NP-hard. Putting these together, 
Theorem~\ref{thm-rcw-gen} follows. 
As the complementary problem 
is \NP-complete, $k$-\rcw generation 
for a single node $v$ is co-\NP-hard. 
Hence the general problem of $k$-\rcw generation  
for a set of test node $V_T$ in a given 
configuration is co-\NP-hard. 
\end{proof}

\eat{
\stitle{Procedure~\kw{PrioritizeQ}$(Q, C, G_s)$}. 
We provide a detailed description of 
the procedure \kw{PrioritizeQ}. 
%\warn{add a 
%paragraph here. 
%No need to give pseudocode.}
}

%\stitle{Minimality of $k$-\rcws}. 
%\warn{Give a description of the algorithm; 
%put correctness and time cost analysis. }

\subsection{Parallel Generation of Robust Explanations}

\stitle{Proof of Lemma~\ref{lm-parallel}}. 
{\em Given a subgraph $G_i$ of $G\setminus G_s$, 
If there is a $j$-disturbance $E^i_j$ 
in $G_i\setminus G_s$, and applying $E^i_j$ 
to $G$ changes the 
result $M(v,G)$ = $l$, then 
$G_s$ is not a $k$-\rcw for 
$M(v,G)$=$l$, for any $k\geq j$.} 

\eat{
Given graph $G$, a set of test nodes 
$V_T$ and a fixed deterministic \gnn $M$, 
a $k$-\rcw for $V_T$ is a $k'$-\rcw for $V_T'$, for any $k'\in[0,k]$ and any 
subset $V_T'\subseteq V_T$. 
}

\begin{proof}
First, $G_s$ is not a $k$-\rcw if 
it is already verified not a witness or 
\cw for $G$. Let $G_s$ be a \cw 
for $M(v, G)$ = $l$. 
Assume there is a $j$-disturbance $E^i_j$ $j\leq k$ 
in a subgraph $G_i$ of $G \setminus G_s$, such that 
$E^i_j$ already serves as a $j$-disturbance 
of $v\in V_T$ such that $M(v,\widetilde{G})$ = $c\neq l$ 
, where $\widetilde{G}$ is obtained by applying the 
$j$-disturbance on $G_i$ alone. Note that  
$G_i\setminus G_s$ = $G_i$, as $G_i$ and $G_s$ 
do not share edges. Hence 
$E^i_j$ is a $j$-disturbance that 
leads to a graph $\widetilde{G}$ in which 
$G_s$ is not a $j$-robust \cw 
for $M(v,G)$=$l$ by definition. 
That is, 
%Given Lemma~\ref{lm-k}, 
$G_s$ is ``disapproved'' by a local 
$j$-disturbance from a  
subgraph $G_i$ at a worker 
$i$ already. Hence $G_s$ 
is not a $j$-\rcw for $G$ for 
$M(v,G)$=$l$. Given Lemma~\ref{lm-k}, 
it is not a $k$-\rcw for any $k\geq j$. 
\end{proof} 

The above result verifies an early-termination condition: during the parallel verification of $G_s$, 
whenever a small disturbance within a budget $k$ 
that can change the label of $M(v,G)$ = $l$ 
is reported by a worker $i$, the parallel verification of 
$G_s$ over other workers can be early terminated. This 
will reduce the parallel communication 
and verification cost.

\stitle{Parallel cost}. 
For the total parallel time cost, 
there are at most $k|V_T|$ rounds 
of parallel computation, and 
$2k|V_T|$ rounds of 
communications between 
the coordinator 
and the workers. In 
each communication, 
(1) \paraexpand incurs on average 
$\frac{|G^i_{s_j}|}{n}$ parallel time cost 
and a data shipment of $\frac{|B_j|+|G^i_{s_j}|}{n}$. 
and (2) \paraverifyrcw incurs a parallel time cost 
in $O(\frac{|B_j|(L|E|F+L|V|F^2)}{n})$ 
time, with a data shipment of $\frac{|B_j|}{n}$. % \textcolor{red}{[AK: unclear sentence]}
Thus the total time cost (including communication cost) is in 
$O(\frac{|G|+|B|)(L|E|F+L|V|F^2)}{n} + I_0\cdot L|E|F+L|V|F^2)$. 
Here $I_0$ refers to the number of $k$-disturbances 
verified at the coordinator site, 
which is disjoint with any verified counterparts from 
any local site; that is, \prcwgen~{\em avoids} 
unnecessary redundant verification. 
This analysis verifies that \prcwgen 
scales well as more 
processors are used. 

%\section{Additional Experiments}

\eat{
\stitle{Proof of Theorem~\ref{thm-feasible}}. 
Given a configuration $C$ 
that specifics $G$, $\M$, 
$V_T$ and $k$, 
there is an algorithm that 
generates a $k$-\rcw in 
$O((N+|G|)(L|E|F+L|V|F^2)$ time, where $N$ is the 
total number of verified $k$-disturbances. 
Specifically for \ppnps under
$(k,b)$-disturbances, 
it computes a $k$-\rcw in $O(kbLF(|E|+|V|F) + k|V_T|)$ time. 

As a constructive proof, it suffices for us to 
present the detailed correctness and time cost 
analysis for the Algorithm~\mrcwgen.

\stitle{Correctness of~\mrcwgen}. 
Algorithm~\mrcwgen always terminates with 
either a non-trivial $k$-\rcw, or trivial cases. 
For the time cost, (1) it takes a total verification cost 
in $O(N\times I)$ 
(line~4), where $N$ is the total number of $k$-disturbances 
being verified, and $I$ is the \gnn-specific 
single inference cost, which is typically bounded in  
$O(L|E|F+L|V|F^2)$ for representative \gnns
(\eg \gcns, \gats, \gsage, \ppnps)~\cite{chen2020scalable,zhou2021accelerating}. 
Procedure~\kw{Expand} takes
$O(|G|I)$ time, as $G_s$ grows at most $|V|+|E|$ times\footnote{Note that although the growth considers node pairs in 
$|V|\times|V|$, $G_s$ does not 
re-add node pairs and grows up to size $|G|$.}. 
The total cost is thus in $O((N+|G|)L|E|F+L|V|F^2)$, 
for representative \gnns. 

Specifically for \ppnps, the algorithm~\mrcwgen 
invokes procedure~\verifyrcwp to 
verify at most $k\times b$ $(k,b)$-disturbances 
for each node $v\in V_T$, and for each verification, 
takes time $O(L|E|F+L|V|F^2)$ for $L$-layered 
\ppnps with $F$ features per node. 
Thus the total verification cost is in 
$O(kbLF(|E|+|V|F))$. Observe that 
the optimal node pairs $E^*_k$ of size $k$ 
for a node 
$v$ only needs to be computed once in 
\verifyrcwp (line~11) or by \kw{Expand} (line~6) via a 
deterministic process, hence 
the procedure\kw{Expand} {\em does not} incur 
additional verification, and incurs a total cost in 
$O(k|V_T|)$. Thus the total cost is in 
$O(kbLF(|E|+|V|F) + k|V_T|)$. 
%Here $b$ is bounded by node degree, and $L$ is 
%typically small for \gnns.  

\vspace{.5ex}
Given the above analysis, Lemma~\ref{thm-rcw-gen-tractable} and Theorem~\ref{thm-feasible} follow. 
 
\stitle{Proof of Lemma~\ref{thm-rcw-gen-tractable}}. 
\warn{This will be a short paragraph just to highlight the time cost analysis of }
}
